# Supplementary material for: Variable Metric Proximal Gradient Method with Diagonal Barzilai-Borwein Stepsize
Source: arXiv:1910.07056 source file (2019-10-15)
Supplement: Supplementary file 1 [file 031consensus_supp.tex]

% !TEX root = icml_vmpg.tex
\begin{algorithm}%[!t]
	\caption{VM-PG for consensus optimization}
	\label{algorithm:consensus}
\begin{algorithmic}
	\STATE {\bfseries given} a starting point $x^0 \in \dom{f}$ 
   \REPEAT
   \FOR{ node $j=1$ {\bfseries to} ${N_{\mathrm{node}}}$}
     \STATE Update metric $U^k_j$ on node $j$
     \STATE $y^{k+1}_j = x^k_j - (U^k_j)^{-1} \nabla f(x^k_j)$
   \ENDFOR
   \STATE $\begin{aligned} z^{k+1} = \left(\sum_{j=1}^{N_{\mathrm{node}}} U_j x_j\right) \bigg/ \left(\sum_{j=1}^{N_{\mathrm{node}}} U_j\right)  \quad \text{(elementwise division)}
   \end{aligned}$
   \FOR{ node $i=1$ {\bfseries to} ${N_{\mathrm{node}}}$}
   		\STATE $x_j^k=z^k$
   \ENDFOR 
   \STATE Do linesearch until \eqref{eq:linesearch} is satisfied
   \UNTIL{stopping criterion $\twonorm{y^{k+1}- y^{k} }\leq \mathrm{\epsilon_{tol}}$ satisfied }
\end{algorithmic}
\end{algorithm}
\subsection{5.1 Metric selections for consensus optimization}
\subsubsection{Global BB-type stepsize} Equation \eqref{prob:consensus} can be represented in its canonical form \eqref{cvxopt_composition} as:- $f(x) = \sum_{j=1}^{N_{\mathrm{node}}} f_j(x_j)$ and $g(x)=\delta_{\mathcal{C}}(x_1, \ldots, x_{N_{\mathrm{node}}})$ for $x = \{x_1,\ldots, x_{N_{\mathrm{node}}}\} \in \reals^{{N_{\mathrm{node}}}n}$. Following Section \ref{sec:metric}, the \textit{scalar} \eqref{eq:bb_hybrid} and \textit{diagonal} \eqref{eq:dbb_solution} BB stepsizes can be computed by referring to global information, i.e., $\{x_j,f_j(x_j) \}_{j=1}^{N_{\mathrm{node}}}$. Thus, for the rest of this section we will refer to these as $\alpha_{\text{global BB}}^k(s^k, y^k)$ and $U_{\text{global DBB}}^k(s^k, y^k)$ respectively. %\youngsuk{one line more}
%However, for both these cases, computing \eqref{eq:bb12} requires global information, i.e., $\{x_j,f_j(x_j) \}_{j=1}^M$. For the rest of this section we will refer to these two approaches in \eqref{eq:bb_hybrid} and \eqref{eq:dbb_solution} as $\alpha_{\text{global BB}}^k(s^k, y^k)$ and $U_{\text{global DBB}}^k(s^k, y^k)$ respectively. However, for consensus problems computing such global stepsizes can be disadvantageous, due to the communication overhead between several agents (nodes). 

\subsubsection{Local BB-type stepsize}
We can extend this into the new \textit{local BB}-type methods. The main idea stems from that the each node approximates its Hessian $\nabla^2 f_j(x_j^k)$ separately, only based on its node (or local) information, i.e., local step $s_j^k = x_j^k - x_j^{k-1}$ and local gradient change $y_j^k = \nabla f_j(x_j^k) - \nabla f(x_j^{k-1})$. This metric selection is well-suited for the observation in the remark above.

\xhdr{Local scalar BB step-size} Each node evaluates $U_j^k = \alpha_{\mathrm{BB}}(s_j^k, y_j^k)I$ from \eqref{eq:bb_hybrid}, only based on local $s_j^k $ and $y_j^k$. Then, the overall diagonal metric is given as
\begin{align} \label{eq::localBB}
U^k_{\mathrm{local~BB}} = \text{blkdiag}(U_{1}^k, \ldots, U_{N_{\mathrm{node}}}^k)	.
\end{align}
\xhdr{Local diagonal BB step-size} Similarly, each node evaluates $U_j^k:= U_{\mathrm{DBB}}(s_j^k, y_j^k)$ using \eqref{eq:dbb_solution}, only based on local $s_j^k $ and $y_j^k$. Then, the overall diagonal metric is given as
\begin{align} \label{eq::localDBB}
U^k_{\mathrm{local~DBB}} = \text{blkdiag}(U_{1}^k, \ldots, U_{N_{\mathrm{node}}}^k)	.
\end{align}

Similarly, we do linesearch (Algorithm \ref{algorithm:metric_selection}) for initial $U^k_{\mathrm{local~BB}}$ and $ U^k_{\mathrm{local~DBB}}$.  

\subsection{5.2 Proximal mapping for consensus optimization }
The standard proximal operation with global BB stepsize on $g(x)$ is the equally weighted average of the local variables $\{x_j\}_{j=1}^{N_{\mathrm{node}}}$ \cite{parikh2014proximal}. However, in VM-PG with diagonal metric $U = \text{Blkdiag}(U_1,\ldots,U_{N_{\mathrm{node}}})$ (such as $U_{\mathrm{global~DBB}}$,$U_{\mathrm{local~BB}}$,and $U_{\mathrm{local~DBB}}$), its scaled proximal step is a weighted average of the local variable weighted by the node metric $U_j$, i.e.,  
\begin{align*}
% 	\left(\prox_{g,U^k_{\mathrm{local~BB}}}(x)\right)_j &= \frac {\sum_{j=1}^M \alpha_j^k x_j}{\sum_{j=1}^M \alpha_j^k},\\
	\left(\prox_{g,U_{\mathrm{j}}}(x)\right)_j &= \left(\sum_{j=1}^{N_{\mathrm{node}}} U_j x_j\right) \bigg/ \left(\sum_{j=1}^{N_{\mathrm{node}}} U_j\right), 
% 	\left(\prox_{g,U^k_{\mathrm{local~DBB}}}(x)\right)_j &= \left(\sum_{j=1}^M U_j x_j\right) \bigg/ \left(\sum_{j=1}^M U_j\right), 
\end{align*}
where the division is coordinate-wise. Then we have the Algorithm \ref{algorithm:consensus}

For example of local BB stepsize, $(\prox_{g,U^k_{\mathrm{local~BB}}}(x))_j = (\sum_{j=1}^M U_j x_j) / (\sum_{j=1}^M U_j)$.

This proximal step makes much more sense in some sense. In first case, suppose all the function types $f_j$ are the same but agent 1 has more data than agent 2. Then, intuitively, the consensus step (proximal step) should weigh $x_1^k$ more than $x_2^k$ to be averaged, rather than treating them equally. Especially when local loss function is proportional to number of data like regression problems and so does its local hessian accordingly, the agent with larger size of data is likely to have larger local metric (stepsize) that is a hessian approximation, being weighted in consensus step. Second, assume types of loss functions over agents are different. Then the scales of local hessians may vary and so do local stepsizes \youngsuk{TODO}.
